# Supplementary material for: Optimal Symmetric Strategies in Multi-Agent Systems with Decentralized Information
Source: arXiv:2307.07150 source file (2023-07-14)
Supplement: Supplementary file 1 [file AppendixA.tex]

\section{Proof of Lemma \ref{LEM:INDEPEN}}
\label{proof:CI1}
We prove the lemma by induction. At $t=1$, the lemma is trivially true since there is no common information at this point and the agents' initial states are independent.

\emph{Induction hypothesis:} Equation \eqref{eq:indepen} holds at time $t$. 
%i.e., for any realization ${x}_{1:t}, {u}_{1:t-1}$ of states and actions, we have
%\begin{align}
% \prob({x}_{1:t},{u}_{1:t-1}|c_t)=\displaystyle\prod_{i=1}^{2} \prob(x^{i}_{1:t},{u}^{i}_{1:t-1}|c_t), 
%\end{align}

\emph{Induction step:} 
Using the induction hypothesis at time $t$, we prove \eqref{eq:indepen} at time $t+1$. In order to do so, it suffices to show that the left hand side of \eqref{eq:indepen} can be factorized as follows:
\begin{align}
\prob({x}_{1:t+1}|c_{t+1}) = \chi^1({x}^1_{1:t+1},c_{t+1})\chi^2({x}^2_{1:t+1},c_{t+1}),\label{factor}
\end{align}
 where $\chi^1$ and $\chi^2$ are some real-valued mappings with $\chi^i$ depending only on agent $i$'s strategy. We establish \eqref{factor} below.
 
 Recall that $c_{{t}+1} = (c_{t},u_{t})$, $I^i_{{t}+1}=(x^i_{1:t+1},u_{1:t})$ and $I^i_{{t}}=(x^i_{1:t}u_{1:t-1})$. Also, note that because of the induction hypothesis at time $t$ and the fact that the randomization at each agent is done independently, we can show that 
 \begin{equation}
   \prob(u_t|c_t) =  \prob(u^1_t|c_t)\prob(u^2_t|c_t).
 \end{equation}
 Now, the left hand side of \eqref{factor} for $t+1$ can be written as

\begin{align}
 &\prob(x_{1:t+1}|c_{t+1})=\frac{\prob(x_{t+1}|x_{1:t},c_{t+1})\prob(u_t|x_{1:t},c_t)\prob(x_{1:t}|c_{t})}{\prob(u_t|c_t)}  \notag\\
 &=\prob(x^{2}_{t+1}|x^{1}_{t+1},x_{1:t},c_{t+1})\prob(x^1_{t+1}|x_{1:t},u_{1:t},c_{t+1})\notag\\
&\quad\times\frac{\prob(u^1_t|x^1_{1:t},c_t)\prob(u^2_t|x^2_{1:t},c_t)\prob(x_{1:t}|c_{t})}{\prob(u^1_t|c_t)\prob(u^2_t|c_t)} \notag \\
 &=\frac{\left[\prob(x^{1}_{t+1}|x^1_{t},c_{t+1})\prob(u^1_t|x^1_{1:t},c_t)\prob(x^1_{1:t}|c_{t})\right]}{\prob(u^1_t|c_t)}\notag\\
 &\quad\times\frac{\left[\prob(x^{2}_{t+1}|x^2_{t},c_{t+1})\prob(u^2_t|x^2_{1:t},c_t)\prob(x^2_{1:t}|c_{t})\right]}{\prob(u^2_t|c_t)}, \label{lnn1:inductive}
\end{align}
where the last equation follows from the state dynamics in \eqref{eq:dyna} and the equation \eqref{eq:indepen} at time $t$. The right hand side of  \eqref{lnn1:inductive} is in the form required by \eqref{factor}. Thus, the induction hypothesis holds at time $t+1$ and the lemma is proved.

% Therefore, by induction, we can conclude that Lemma \ref{LEM:INDEPEN} holds at all times.
