# Supplementary material for: Optimal Symmetric Strategies in Multi-Agent Systems with Decentralized Information
Source: arXiv:2307.07150 source file (2023-07-14)
Supplement: Supplementary file 2 [file AppendixB.tex]

\section{Proof of Theorem \ref{PROP:ONE}}\label{proponeproof}
We will prove the theorem using the following claim.
\begin{claim}\label{claim:one}
 Consider any arbitrary symmetric strategy pair $(g,g)$ for the team. Then there exists a strategy pair $(\bar{g}, \bar{g})$ for the team such that for each $t$, $\bar{g}_t$ is a function of $X_t^i$ and $C_t$ and 
\[
J(\bar{g},\bar{g}) = J(g,g).
\]

%\emph{for every strategy $g^2 \in \mathcal{G}^2$.}
\end{claim}

Suppose that the above claim is true. Let $(g',g')$ be an \emph{optimal symmetric strategy pair} for the team.
Due to Claim \ref{claim:one}, there exists a strategy pair  $(\bar{g}',\bar{g}')$ for the team such that for each $t$, $\bar{g}'_t$ are functions of $X_t^i$ and $C_t$
\[
J(\bar{g}',\bar{g}') = J(g',g')
\]
Thus, $(\bar{g}',\bar{g}')$ is also an optimal symmetric strategy pair where each agent uses only its current state and common information. This proves Theorem \ref{PROP:ONE}. We now proceed to prove Claim \ref{claim:one}. 

\noindent{\emph{Proof of Claim \ref{claim:one}:}} 
 Let $c_t$ be realization of the common information $C_t$ at time $t$. 
We define the distribution $\Psi_t(c_t)$ over the space $(\X^{t}\times\X^{t}) \times(\U\times\U)$
% $(\prod_{\tau = 1}^t(\X^{\tau}\times\X^{\tau}) \times(\U^{t}\times\U^{t}))$ as follows:
% $(\prod_{\tau = 1}^t\prod_{i=1,2}\X^i_{\tau} \times\prod_{i=1,2}\U_{t}^{i})$ 
as follows:
\begin{align}\label{eq:psi1}
&\Psi_t(c_t; x_{1:t},u_{t})\doteq \prob^{(g,g)}[(X_{1:t},U_t) = (x_{1:t},u_t) \mid C_t=c_t],
\end{align}
Similarly, we define the distribution $\Psi^i_t(c_t)$ over the space $\X^{t} \times\U$ 
% $(\prod_{\tau = 1}^t\X^{\tau} \times\U^{t})$ 
as follows:
\begin{align}\label{eq:psi2}
&\Psi^i_t(c_t; x^i_{1:t},u^i_{t})\doteq \prob^{g}[(X^i_{1:t},U^i_t) = (x^i_{1:t},u^i_t) \mid C_t=c_t]
\end{align}
% if $c_t$ is \emph{feasible}, that is $\prob^{g}[C_t = c_t] > 0$, under the \emph{open-loop} strategy. Otherwise, define $\Psi_t(c_t; x_{1:t},u_{t})$ to be the uniform

%  distribution over the space $(\prod_{\tau = 1}^t\prod_{i=1,2}\X^i_{\tau} \times\prod_{\tau = 1}^{t-1}\prod_{i=1,2}\U_{\tau}^{i})$. 

% \begin{lemma}\label{claimJ1}
% Let $(g,g)$ be the team's strategy. Then for any realization $x_{1:t},u_{1:t},m_{t}$ of the variables $X_{1:t},U_{1:t},M_t$, we have
% \begin{align*}
% &\Py^{f,g,g^a}[X_{1:t},U_{1:t-1},M_t = (x_{1:t},u_{1:t-1},m_t) \mid I_t^a] = \Psi_t(I_t^a; x_{1:t},u_{1:t-1},m_t)\\
% &\Py^{f,g,g^a}[X_{1:t},U_{1:t} = (x_{1:t},u_{1:t}) \mid I_{t^+}^a] = \Psi_{t^+}(I_{t^+}^a; x_{1:t},u_{1:t}),
% \end{align*}
% almost surely.
% \end{lemma}

\begin{corollary}\label{factorcorol}
At any given time $t$, the function $\Psi_t$ can be factorized as
\begin{align}
    &\Psi_{t}(c_t; x_{1:t},u_{t}) = \Psi^1_{t}(c_t; x^1_{1:t},u^1_{t})\times \Psi^2_{t}(c_t; x^2_{1:t},u^2_{t}). 
\end{align}
\end{corollary}
The corollary above  is a direct consequence of the conditional independence property of Lemma \ref{LEM:INDEPEN}.

We also define the distribution $\Phi^i_t(c_t)$ over the space $\X \times \U$ as follows:
\begin{align}
\Phi^i_t(c_t; x^i_t, u^i_t) = {\sum_{x^i_{1:t-1}}\Psi^i_t(c_t;x^i_{1:t},u^i_t)}.\label{eq:phia}
\end{align}
% Note that $\Phi^i_t(c_t)$ is a marginal distribution o

% Using Corollary \ref{factorcorol}, we can say that the functions $\Phi_t$ and $\Phi_{t^+}$ can be factorized as
% \begin{align}
%     \Phi_t(\iota_t^a; x_t, m_t) &= \Phi_t^1(\iota_t^a; x_t^1, m_t^1)\Phi_t^2(\iota_t^a; x_t^2, m_t^2)
   
% \end{align}
% We know that the system dynamics $f_t(.)$ are same for both the agents.

% Consider 
% Define communication strategy $\bar{f}^i$ for agent $i$ in the Team such that for any realization $x_t^i, \iota_t^a$ of state $X_t^i$ and adversary's information $I_t^a$ at time $t$, the probability of selecting an action $m_t^i$ at time $t$ is
% \begin{align}\label{eq:defgbara}
% \bar{f}_t^i(x_t^i,\iota_{t}^a;m_t^i) \doteq 
% \begin{cases}
% \frac{\Phi_t^i(\iota_t^a; x_t^i, m_t^i)}{\sum_{m'_t}\Phi_t^i(\iota_t^a; x_t^i, m'_t)} & \text{if } {\sum_{m'_t}\Phi_t^i(\iota_t^a; x_t^i, m'_t)} > 0\\
% \mathscr{U}(\cdot) & \text{otherwise},
% \end{cases}
% \end{align}
% where $\mathscr{U}(\cdot)$ denotes the uniform distribution over the action space $\{0,1\}$. Notice that the construction of the strategy $\bar{f}^i$ does not involve adversary's strategy $g^a$.

 We now define a control strategy $\bar{g}^1$ for agent $1$ in the team such that for any realization $ c_t$ of common information $C_t$ at time ${t}$ and any realization $x^1$ of the state $X_t^1$, the probability of selecting an action $u^1 \in \mathcal{U}$ at time ${t}$ is\\ \red{Please check the following definitions and superscripts CAREfully}
$\bar{g}^1_{t}(x^1,c_t;u^1) :=$
\begin{equation}\label{eq:defgbar}
   \begin{cases} 
\frac{\Phi_{t}^1(c_t; x^1,u^1)}{\sum_{u'1}\Phi_{t}^1(c_t; x^1,u'^1)} & \text{if } \sum_{u'^1}\Phi_{t}^1(c_t; x^1,u'^1) > 0\\
~& ~\\
\frac{\Phi_{t}^2(c_t; x^1,u^1)}{\sum_{u'^1}\Phi_{t}^2(c_t; x^1,u'^1)} & \text{if } \sum_{u'^1}\Phi_{t}^1(c_t; x^1,u'^1)=0 \\
&\text{and}\sum_{u'^1}\Phi_{t}^2(c_t; x^1,u'^1)>0\\
~& ~\\
\frac{1}{|\mathcal{U}|} &  \text{otherwise},
\end{cases} 
\end{equation}

%\mathscr{U}(\cdot) &  \text{otherwise}
% where $\mathscr{U}(\cdot)$ denotes the uniform distribution over the action space $\U$.
We define a control strategy $\bar{g}^2$ for agent $2$ in a similar way: for any realization $ c_t$ of common information $C_t$ at time ${t}$ and any realization $x^2$ of the state $X_t^2$, the probability of selecting an action $u^2 \in \mathcal{U}$ at time ${t}$ is\\
%Similarly we define $\bar{g}^2_{t}(x_t^2,c_t;u_{t}^2) $.
$\bar{g}^2_{t}(x^2,c_t;u^2) :=$
\begin{align}\label{eq:defgbar2}
\begin{cases} 
\frac{\Phi_{t}^2(c_t; x^2,u^2)}{\sum_{u'^2}\Phi_{t}^2(c_t; x^2,u'^2)} & \text{if } \sum_{u'^{2}}\Phi_{t}^2(c_t; x^2,u'^2) > 0\\
~& ~\\
\frac{\Phi_{t}^1(c_t; x^2,u^2)}{\sum_{u'^2}\Phi_{t}^1(c_t; x^2,u'^2)} & \text{if } \sum_{u'^2}\Phi_{t}^2(c_t; x^2,u'^2)=0 \\
&\text{and}\sum_{u'^2}\Phi_{t}^1(c_t; x^2,u'^2)>0\\
~& ~\\
\frac{1}{|\mathcal{U}|} &  \text{otherwise},
\end{cases}
\end{align}
% \red{INSERT equation numbers for definition of g bar 1 and g bar 2})
The following lemma connects $\bar{g}^1_{t}$ and $\bar{g}^2_{t}$ defined above.
\begin{lemma}\label{samestrategy}
Consider $x^1 =x^2$ and $u^1=u^2$. Then, if 
 both ${\sum_{u'^1}\Phi_{t}^1(c_t; x^1,u'^1)}> 0$ and ${\sum_{u'^2}\Phi_{t}^2(c_t; x^2,u'^2)}> 0$, we have
\begin{align}
    \frac{\Phi_{t}^1(c_t; x^1,u^1)}{\sum_{u'^1}\Phi_{t}^1(c_t; x^1,u'^1)}=\frac{\Phi_{t}^2(c_t; x^2,u^2)}{\sum_{u'^2}\Phi_{t}^2(c_t; x^2,u'^2)}
\end{align}
Consequently, the functions $\bar{g}^1_t: \mathcal{X} \times \mathcal{U}^{t-1} \mapsto \Delta(\mathcal{U})$ and $\bar{g}^2_t: \mathcal{X} \times \mathcal{U}^{t-1} \mapsto \Delta(\mathcal{U})$ are identical.
%control strategy $\bar{g}^1=\bar{g}^2=:\bar{g}$. 
\begin{proof}
See Appendix D.
\end{proof}

\end{lemma}
% For convenience, let us define
% \begin{align}
%     \bar{f}_t(x_t,\iota_t^a;m_t) &= \bar{f}_t^1(x_t^1,\iota_t^a;m_t^1)\bar{f}_t^2(x_t^2,\iota_t^a;m_t^2)\\
%     \bar{g}_t(x_t,\iota_{t^+}^a;u_t) &= \bar{g}_t^1(x_t^1,\iota_{t^+}^a;u^1_t)\bar{g}_t^2(x_t^2,\iota_{t^+}^a;u_t^2).
% \end{align}

Since Lemma \ref{samestrategy} establishes that the functions $\bar{g}^1_t$ and $\bar{g}^2_t$  are identical, we will simply denote them by $\bar{g}_t$ from now on.

\begin{remark}
We note that the distribution $\Phi^i_t(\cdot)$ defined in \eqref{eq:phia} may be  different for the two  agents.  The following example illustrates that: The state space $\mathcal{X}=\{0,1\}$ and the action space $\mathcal{U}=\{0,1\}$.\red{CLEAN up the notation. What is the state space in this example? The action space? What is g? Use FORMAL language in writing and use complete sentences.}
Initial states for both the agents are given by $X^1_1=0$ and $X^2_1=1$.
We assume that the state remains the same for all time $t$. Consider now the following strategy for each agent:
\begin{align}
U^i_t =
\begin{cases}
0 & \text{if } X^i_1=0\\
1 & \text{otherwise } 
\end{cases}
\end{align}
\begin{align}
&\prob^g[X^1_t,U^1_t|C_t=c_t] =
\begin{cases}
1 & \text{if } (X^1_t,U^1_t)=(0,0)\\
0 & \text{otherwise } 
\end{cases}
\end{align}

\begin{align}
&\prob^g[X^2_t,U^2_t|C_t=c_t] =
\begin{cases}
1 & \text{if } (X^2_t,U^2_t)=(1,1)\\
0 & \text{otherwise } 
\end{cases}
\end{align}
It is straightforward to see that $\Phi^1_t(c_t; x^1_t, u^1_t)\neq \Phi^2_t(c_t; x^2_t, u^2_t)$.
\red{I will check remark later}
\end{remark}
% \begin{lemma}\label{aseqstrat}
% At time $t$, we have
% \begin{align*}
% \prob^{g}[U^i_t = u^i_t \mid X^i_t, C_t] = \bar{g}_t(X^i_t,C_{t};u^i_t)
% \end{align*}
% almost surely for every $u^i_t$.
% \end{lemma}
% \begin{proof}
% Let $x^i_{1:t}, c_t$ be a realization that has a non-zero probability of occurrence under the strategy $g$. Then using Lemma \ref{claimJ1}, we have
% \begin{align}
% \prob^{g}[X^i_{1:t},U^i_{t}= (x^i_{1:t},u^i_{t}) \mid c_t] = \Psi_t(c_t; x^i_{1:t},u^i_t), \label{eq:lemma14a}
% \end{align}
% Summing over all $x^i_{1:t-1},u^i_{t}$ and using  \eqref{eq:phia} and \eqref{eq:lemma14a},  we have
% \begin{align}
%  \prob^{g}[X^i_t = x^i_t \mid C_t=c_t] =\sum_{u^i_t}\Phi^i_t(c_t; x^i_t,u^i_t).
% \end{align}
% The left hand side of the above equation is positive since $x_t,c_t$ is a realization of positive probability under the strategy $g$.

% Using Bayes' rule,  \eqref{eq:phia}, \eqref{eq:defgbar} and \eqref{eq:lemma14a}, we obtain
% \begin{align}
% \nonumber\prob^{(g,g)}[U^i_t = u^i_t \mid X^i_t = x^i_t, C_t=c_t]
% &= \bar{g}_t(x^i_t,c_t;u^i_t) .
% \end{align}
% This concludes the proof of the lemma.
% \end{proof}

\begin{lemma}\label{LEM:aseqstrat2}
Let $x^1_{1:t},x^2_{1:t}, c_t$ be  realizations of $X^1_{1:t}, X^2_{1:t}$ and $C_t$ respectively such that $\prob^{(g,g)}(x^1_{1:t},x^2_{1:t}, c_t)>0$. Then, for every $u^1_t \in \mathcal{U}$ and $u^2_t \in \mathcal{U}$,
\begin{align}\label{eq:lemm6}
\prob^{(g,g)}[U^1_t = u^{1}_t, U^2_t=u^2_t &\mid X_t=x^{1,2}_t, C_t=c_t] \notag\\
&=\bar{g}_t(x^1_t,c_{t};u^1_t)\bar{g}_t(x^2_t,c_{t};u^2_t).
\end{align}
%almost surely for every $u^{1,2}_t$.
\end{lemma}
\begin{proof}
Using the  conditional independence property of Lemma \ref{LEM:INDEPEN}, the left hand side of \eqref{eq:lemm6} is equal to 
\begin{align*}
        &\displaystyle\prod_{i=1}^{2}\prob^{g}[U^i_t = u^i_t \mid X^i_t=x^i_t, C_t=c_t].
    % \notag\\
    % &\stackrel{(a)}= \bar{g}_t(X^1_t,C_{t};u^1_t)\bar{g}_t(X^2_t,C_{t};u^2_t)
\end{align*}
% \begin{align*}
%     \prob^{(g,g)}[U_t = u^{1,2}_t &\mid X_t=x^{1,2}_t, C_t=c_t]=\notag\\
%     &\displaystyle\prod_{i=1}^{2}\prob^{g}[U^i_t = u^i_t \mid X^i_t=x^i_t, C_t=c_t]
%     % \notag\\
%     % &\stackrel{(a)}= \bar{g}_t(X^1_t,C_{t};u^1_t)\bar{g}_t(X^2_t,C_{t};u^2_t)
% \end{align*}
% At time $t$, its sufficient to prove that
% \begin{align*}
% \prob^{g}[U^i_t = u^i_t \mid X^i_t=x^i_t, C_t=c_t] = \bar{g}_t(x^i_t,c_{t};u^i_t)
% \end{align*}
% almost surely for every $u^i_t$.\\
% Let $x^i_{1:t}, c_t$ be a realization that has a non-zero probability of occurrence under the strategy $g$.

From equation \eqref{eq:psi2}, we have
\begin{align}
\prob^{g}[(X^i_{1:t},U^i_{t})= (x^i_{1:t},u'^i) \mid C_t = c_t] = \Psi^i_t(c_t; x^i_{1:t},u'^i), \label{eq:lemma14a}
\end{align}
Summing over all $x^i_{1:t-1},u'^i$ and using  \eqref{eq:phia} in \eqref{eq:lemma14a},  we have
\begin{align}\label{eq:lemma6b}
 \prob^{g}[X^i_t = x^i_t \mid C_t=c_t] =\sum_{u'^i}\Phi^i_t(c_t; x^i_t,u'^i).
\end{align}
The left hand side of the above equation is positive since $x^i_t,c_t$ is a realization of positive probability under the strategy $g$. We further note that from \eqref{eq:psi2} and \eqref{eq:phia}, we have
\begin{equation}\label{eq:lemma6a}
     \prob^{g}[X^i_t = x^i_t, U^i_t=u^i_t \mid C_t=c_t] = \Phi^i_t(c_t; x^i_t,u^i_t).
\end{equation}

Dividing \eqref{eq:lemma6a} by \eqref{eq:lemma6b} and using the  definition of $\bar{g}$ (see \eqref{eq:defgbar} and \eqref{eq:defgbar2}), we obtain
% \red{INSERT equation numbers for definition of g bar 1 and g bar 2}),   
\begin{align}
\nonumber\prob^{g}[U^i_t = u^i_t \mid X^i_t = x^i_t, C_t=c_t]
&= \bar{g}_t(x^i_t,c_t;u^i_t) .
\end{align}
This concludes the proof of the lemma.
% For where (a) follows from Lemma \ref{aseqstrat}
\end{proof}

Let $\bar{g} = (\bar{g}_1,\ldots,\bar{g}_T)$.  We can now show that the strategy pair $(\bar{g},\bar{g})$ satisfies
\[
J(\bar{g},\bar{g}) = J({g},{g}).
\]
Because of the structure of the cost function in \eqref{eq:cost2}, it is sufficient to show that for each time $t$, the random variables   $(X_t,U_t,C_t)$ have the same joint distribution under strategy pairs $({g},{g})$ and $(\bar{g},\bar{g})$. We prove this by induction.  It is easy to verify that at time $t=1$, $(X_1,U_1,C_1)$ have the same joint distribution under strategy profiles $({g},{g})$ and $(\bar{g},\bar{g})$.
Now assume that at time $t$, 
\begin{align}
\label{jointeq}\prob^{({g},{g})}[x_t,u_t,c_t] = \prob^{(\bar{g},\bar{g})}[x_t,u_t,c_t],
\end{align}
for any realization of state, actions and common information $x_t,u_t,c_t$. Consider   any realization $x_{t+1},u_{t+1},c_{t+1}$ that has non-zero probability of occurrence under the strategy profile ${({g},{g})}$. Then, since $c_{t+1}=(c_t,u_t)$, we have
\begin{align}
&\prob^{({g},{g})}[x_{t+1},c_{t+1}] =\sum_{\bar{x}_t} \prob[x_{t+1}\mid {\bar{x}_t},u_t]\prob^{({g},{g})}[\bar{x}_t,u_t,c_{t}] \notag \\
% &=\sum_{\bar{x}_t}\prob[x^1_{t+1}\mid {\bar{x}^1_t},u_t]\prob[x^2_{t+1}\mid {\bar{x}^2_t},u_t]\prob^{(\bar{g},\bar{g})}[\bar{x}_t,u_t,c_{t}]\\
&=\prob^{(\bar{g},\bar{g})}[x_{t+1},c_{t+1}].\label{indhyp}
\end{align}
% Now assume that at time $t^+$, 
% \begin{align}
% \label{jointeq}\Py^{(({f},{g}),g^a)}[x_t,u_t,u_t^a,\iota_{t^+}^a] = \Py^{((\bar{f},\bar{g}),g^a}[x_t,u_t,u_t^a,\iota_{t^+}^a],
% \end{align}
%  for any realization of state, actions and adversary's information $x_t,u_t,u_t^a,\iota_{t^+}^a$. Let $\iota_{t+1}^a = (\iota_{t^+}^a,u^a_t,x^0_{t+1})$. Then we have
% \begin{align}
% \Py^{(({f},{g}),g^a)}[x_{t+1},\iota_{t+1}^a] &= \nonumber\sum_{\bar{x}_t}\sum_{\bar{u}_t}\Py[x_{t+1},x_{t+1}^0 \mid \bar{x}_t,\bar{u}_t,u_t^{a},\iota_{t^+}^a]\Py^{(({f},{g}),g^a)}[\bar{x}_t,\bar{u}_t,u_t^{a},\iota_{t^+}^a]\\
% &= \label{indhyp}\sum_{\bar{x}_t}\sum_{\bar{u}_t}\Py[x_{t+1},x_{t+1}^0 \mid \bar{x}_t,\bar{u}_t,u_t^{a},\iota_{t^+}^a]\Py^{((\bar{f},\bar{g}),g^a}[\bar{x}_t,\bar{u}_t,u_t^{a},\iota_{t^+}^a]\\
% &=\Py^{((\bar{f},\bar{g}),g^a}[x_{t+1},\iota_{t+1}^a].\label{indhyp2}
% \end{align}
The equality in (\ref{indhyp}) is due to the system dynamics and induction hypothesis.
% At $t+1$, for any realization $x_{t+1},u_{t+1},c_{t+1}$ that has non-zero probability of occurrence under the strategy profile ${({g},{g})}$, 
Further, we have
\begin{align}\label{constarg}
&\prob^{({g},{g})}[x_{t+1},u_{t+1},c_{t+1}]\notag \\
&= \prob^{({g},{g})}[u_{t+1}\mid x_{t+1},c_{t+1}]\prob^{({g},{g})}[x_{t+1},c_{t+1}]\\
&=\bar{g}_t(x^1_{t+1},c_{t+1};u^1_{t+1})\bar{g}_t(x^2_{t+1},c_{t+1};u^2_{t+1})\times\notag\\
&\prob^{({g},{g})}[x_{t+1},c_{t+1}]\label{constarg1}
\end{align}
\begin{align}
&= \prob^{(\bar{g},\bar{g})}[u_{t+1}\mid x_{t+1},c_{t+1}]\prob^{(\bar{g},\bar{g})}[x_{t+1},c_{t+1}]\label{constarg3}\\
&= \prob^{(\bar{g},\bar{g})}[x_{t+1},u_{t+1},c_{t+1}]\label{constarg4},   
\end{align}
where the equality in \eqref{constarg} is a consequence of the chain rule and the manner in which players randomize their actions. 
% \red{Please combine the previous equation - eqn 51-  and the ones below into one block and move explanations of all steps at the end}
Equality in \eqref{constarg1} follows from Lemma \ref{LEM:aseqstrat2} and the equality in \eqref{constarg3} follows from the result in \eqref{indhyp}.
 Therefore, by induction, the equality in \eqref{jointeq} holds for all $t$. Hence, the expected costs at each time are the same under strategy pairs $(g,g)$ and $(\bar{g}, \bar{g})$. This concludes the proof of Claim \ref{claim:one}. \qed
