# Supplementary material for: Optimal Symmetric Strategies in Multi-Agent Systems with Decentralized Information
Source: arXiv:2307.07150 source file (2023-07-14)
Supplement: Supplementary file 3 [file AppendixC.tex]

\section{Proof of Lemma \ref{LEM:UPDATE}}\label{proof:Coordd}
To prove Lemma \ref{LEM:UPDATE} we use the conditional independence property results from  \cite{mahajan2013optimal}.
For Problem P1b, the conditional independence proposition 1 of \cite{mahajan2013optimal} applies directly and is given by:
\begin{equation}\label{eq:indepen}
    \prob^{(g,g)}({x}_{1:t}|c_t)=\displaystyle\prod_{i=1}^{2} \prob^{g}(x^{i}_{1:t}|c_t), 
\end{equation}
% Recall that at the beginning of time $t$, the common information is given by $C_{t}:=(Z^{er}_{1:t-1},M^{1,2}_{1:t-1})$ (see \eqref{commoninfo}).
% At the end of time $t$, i.e. after the communication decisions are made at time $t$, the common information is given by $C_{t^+}:=(Z^{er}_{1:t},M^{1,2}_{1:t})$ (see \eqref{commoninfoplus}). 
Let $c_{t} := u_{1:t-1}$ and $c_{t+1} := u_{1:t}$ be realizations of $C_t$, $C_{t+1}$ respectively. Let $\gamma_{1:t}$ be the realizations of the coordinator's prescriptions $\Gamma_{1:t}$ up to time $t$. Let us assume that the realizations $c_{t+1},\gamma_{1:t}$ have non-zero probability. Let $\pi^i_t$ and $\pi^i_{t+1}$ be the corresponding realizations of the coordinator's beliefs $\Pi^i_t$ and $\Pi^i_{t+1}$ respectively for $i=1,2$. These beliefs are given by
\begin{align}
&\pi^i_{t}(x^i_t)=\prob(X^i_t=x^i_t|C_t=u_{1:t-1},\Gamma_{1:t-1}=\gamma_{1:t-1})\notag\\
    &\pi^i_{t+1}(x^i_{t+1})=\prob(X^i_{t+1}=x^i_{t+1}|C_{t+1}=u_{1:t},\Gamma_{1:t}=\gamma_{1:t}).\notag
\end{align}
Let $\mathscr{P}^i_{t}$ be defined as the probability of $x^i_{t+1},x_t,u_t$ conditioned on the realizations $c_t$, $\gamma_{1:t}$ of common information $C_t$ and prescriptions $\Gamma_{1:t}$ at time $t$.
\begin{align}
\mathscr{P}^i_{t}(c_t,\gamma_{1:t};x^i_{t+1},x_t,u_t):=\prob(x^i_{t+1},x_t,u_t|u_{1:t-1},\gamma_{1:t}).\label{def:lemma4bayes}
\end{align}
Using Bayes' rule, we have 
\begin{align}\label{eq:bayesupdate4}
    \pi^i_{t+1}(x^i_{t+1})=&\prob(X^i_{t+1}=x^i_{t+1}|u_{1:t},\gamma_{1:t})\notag\\
    =&\frac{\prob(X^i_{t+1}=x^i_{t+1},U_t=u_t|u_{1:t-1},\gamma_{1:t})}{\prob(U_t=u_t|u_{1:t-1},\gamma_{1:t})}\notag\\
    =&\frac{\sum_{x_t}\mathscr{P}^i_{t}(c_t,\gamma_{1:t};x^i_{t+1},x_t,u_t)}{\sum_{x^i_{t+1}}\sum_{x_t}\mathscr{P}^i_{t}(c_t,\gamma_{1:t};x^i_{t+1},x_t,u_t)}
  \end{align}  
  Consider equation \eqref{def:lemma4bayes}, which can be further simplified into:
  \begin{align}\label{eq:bayesupdate41}
  &\mathscr{P}^i_{t}(c_t,\gamma_{1:t};x^i_{t+1},x_t,u_t)\notag\\
    %   &=\prob(x^1_{t+1}|x^1_t,u_t)\prob(x^2_{t+1}|x^2_t,u_t)\gamma_t(x^1_t;u^1_t)\gamma_t(x^2_t;u^2_t)\notag\\
    %   &\times \prob(x_t|u_{1:t-1},\gamma_{1:t})\notag\\
    %   &\stackrel{(a)}{=}\prob(x^1_{t+1}|x^1_t,u_t)\prob(x^2_{t+1}|x^2_t,u_t)\gamma_t(x^1_t;u^1_t)\gamma_t(x^2_t;u^2_t)\prob(x_t|u_{1:t-1},\gamma_{1:t-1})\notag\\
    &=\prob(x^i_{t+1}|x^i_t,u_t)\gamma_t(x^1_t;u^1_t)\gamma_t(x^2_t;u^2_t)\pi^1_{t}(x^1_t)\pi^2_{t}(x^2_t)
    %   &=\prob(x^1_{t+1}|x^1_t,u_t)\prob(x^2_{t+1}|x^2_t,u_t)\gamma_t(x^1_t;u^1_t)\gamma_t(x^2_t;u^2_t)\pi_{t}(x_t)
  \end{align}
  \begin{align}\label{eq:bayesupdate42}
  \frac{\sum_{x^1_t}\prob(x^1_{t+1}|x^1_t,u_t)\gamma_t(x^1_t;u^1_t)\pi^1_{t}(x^1_t)\sum_{x^2_t}\gamma_t(x^2_t;u^2_t)\pi^2_{t}(x^2_t)}{\sum_{x^1_{t+1}}\sum_{x^1_t}\prob(x^1_{t+1}|x^1_t,u_t)\gamma_t(x^1_t;u^1_t)\pi^1_{t}(x^1_t)\sum_{x^2_t}\gamma_t(x^2_t;u^2_t)\pi^2_{t}(x^2_t)}
  \end{align}
  \begin{align}\label{eq:bayesupdate42}
  =\frac{\sum_{x^1_t}\prob(x^1_{t+1}|x^1_t,u_t)\gamma_t(x^1_t;u^1_t)\pi^1_{t}(x^1_t)}{\sum_{x^1_{t+1}}\sum_{x^1_t}\prob(x^1_{t+1}|x^1_t,u_t)\gamma_t(x^1_t;u^1_t)\pi^1_{t}(x^1_t)}
  \end{align}
 Therefore the belief update equation \eqref{eq:bayesupdate4} using equation 
   \eqref{eq:bayesupdate41} for $i=1,2$, can be written as
%   \begin{align}
%       \pi^i_{t+1}=\eta^i_t( \pi^1_{t},\pi^2_{t},\gamma_t,u_t)
%   \end{align}
 \begin{align}
      \pi^1_{t+1}=\eta^1_t( \pi^1_{t},\gamma_t,u_t)
  \end{align}
  \begin{align}
      \pi^2_{t+1}=\eta^2_t( \pi^2_{t},\gamma_t,u_t)
  \end{align}
We denote the belief update equation using $\eta^i_t$.
