# Supplementary material for: Optimal Symmetric Strategies in Multi-Agent Systems with Decentralized Information
Source: arXiv:2307.07150 source file (2023-07-14)
Supplement: Supplementary file 4 [file AppendixC2.tex]

\section{Proof of Lemma \ref{LEM5:UPDATE}}\label{proof2:Coordd}
Let $c_{t} := u_{1:t-1},z_{1:t}$ and $c_{t+1} := u_{1:t},z_{1:t+1}$ be realizations of $C_t$, $C_{t+1}$ respectively. Let $\sigma_{1:t}$ be the realizations of the coordinator's prescriptions $\Sigma_{1:t}$ up to time $t$. Let us assume that the realizations $c_{t+1},\sigma_{1:t}$ have non-zero probability. Let $\lambda^i_t$ and $\lambda^i_{t+1}$ be the corresponding realizations of the coordinator's beliefs $\Lambda^i_t$ and $\Lambda^i_{t+1}$ respectively for $i=1,2$. These beliefs are given by
\begin{align}
&\lambda^i_{t}(x^i_{1:t})=\prob(X^i_{1:t}=x^i_{1:t}|C_t=u_{1:t-1},z_{1:t},\Sigma_{1:t-1}=\sigma_{1:t-1})\notag\\
    &\lambda^i_{t+1}(x^i_{1:t+1})=\notag\\
    &\prob(X^i_{1:t+1}=x^i_{1:t+1}|C_{t+1}=u_{1:t},z_{1:t+1},\Sigma_{1:t}=\sigma_{1:t}).\notag
\end{align}
% Let $\mathscr{P}^i_{t}$ be defined as the probability of $x^i_{t+1},x_t,u_t$ conditioned on the realizations $c_t$, $\gamma_{1:t}$ of common information $C_t$ and prescriptions $\Gamma_{1:t}$ at time $t$.
% \begin{align}
% \mathscr{P}^i_{t}(c_t,\gamma_{1:t};x^i_{t+1},x_t,u_t):=\prob(x^i_{t+1},x_t,u_t|u_{1:t-1},\gamma_{1:t}).\label{def:lemma4bayes}
% \end{align}
Using Bayes' rule, we have 
\begin{align}\label{eq:bayesupdat2}
    &\lambda^i_{t+1}(x^i_{1:t+1})=\prob(X^i_{1:t+1}=x^i_{1:t+1}|u_{1:t},z_{1:t+1},\sigma_{1:t})\notag\\
    =&\frac{\sum_{x^{-i}_{1:t}}\prob(X^i_{1:t+1}=x^i_{1:t+1},x^{-i}_{1:t},u_{1:t},z_{1:t+1},\sigma_{1:t})}{\sum_{x^i_{1:t+1}}\sum_{x^{-i}_{1:t}}\prob(x^i_{1:t+1},x^{-i}_{1:t},u_{1:t},z_{1:t+1},\sigma_{1:t})}\notag\\
    % =&\frac{\sum_{x_t}\mathscr{P}^i_{t}(c_t,\gamma_{1:t};x^i_{t+1},x_t,u_t)}{\sum_{x^i_{t+1}}\sum_{x_t}\mathscr{P}^i_{t}(c_t,\gamma_{1:t};x^i_{t+1},x_t,u_t)}
  \end{align}  
%   Let $\mathscr{P}^i_{t}$ be defined as the joint probability of $x^i_{1:t+1},x^{-i}_{1:t},u_{1:t},z_{1:t+1},\sigma_{1:t}$  at time $t$.
% \begin{align}
% \mathscr{P}^i_{t}(x^i_{1:t+1},x^{-i}_{1:t},u_{1:t},z_{1:t+1},\sigma_{1:t}):=\prob(x^i_{1:t+1},x^{-i}_{1:t},u_{1:t},z_{1:t+1},\sigma_{1:t}).\label{def:lemma4bayes2}
% \end{align}
  Consider numerator of equation \eqref{eq:bayesupdat2} for agent $1$, which can be further simplified into:
  \begin{align}\label{eq:bayesupdate421}
  &\sum_{x^2_{1:t}}\prob(x^1_{1:t+1},x^{2}_{1:t},u_{1:t},z_{1:t+1},\sigma_{1:t})=\notag\\
    &\sum_{x^2_{1:t}}\alpha(x^1_{t+1})\prob(z_{t+1}|z_t,u_t)\sigma_t(x^1_{1:t};u^1_t)\sigma_t(x^2_{1:t};u^2_t)\lambda^1_{t}(x^1_{1:t})\lambda^2_{t}(x^2_{1:t})
  \end{align}
  Consider equation \eqref{eq:bayesupdat2},
%   \begin{align}\label{eq:bayesupdate422}
%   &\frac{\alpha(x^1_{t+1})\prob(z_{t+1}|z_t,u_t)\sigma_t(x^1_{1:t};u^1_t)\lambda^1_{t}(x^1_{1:t})\sum_{x^2_{1:t}}\sigma_t(x^2_{1:t};u^2_t)\lambda^2_{t}(x^2_{1:t})}{\sum_{x^1_{1:t+1}}\alpha(x^1_{t+1})\prob(z_{t+1}|z_t,u_t)\sigma_t(x^1_{1:t};u^1_t)\lambda^1_{t}(x^1_{1:t})\sum_{x^2_{1:t}}\sigma_t(x^2_{1:t};u^2_t)\lambda^2_{t}(x^2_{1:t})}\notag\\
%   &\frac{\alpha(x^1_{t+1})\prob(z_{t+1}|z_t,u_t)\sigma_t(x^1_{1:t};u^1_t)\lambda^1_{t}(x^1_{1:t})}{\sum_{x^1_{1:t+1}}\alpha(x^1_{t+1})\prob(z_{t+1}|z_t,u_t)\sigma_t(x^1_{1:t};u^1_t)\lambda^1_{t}(x^1_{1:t})}\notag\\
%   &=\alpha(x^1_{t+1})\times\frac{\prob(z_{t+1}|z_t,u_t)\sigma_t(x^1_{1:t};u^1_t)\lambda^1_{t}(x^1_{1:t})}{\sum_{x^1_{1:t}}\prob(z_{t+1}|z_t,u_t)\sigma_t(x^1_{1:t};u^1_t)\lambda^1_{t}(x^1_{1:t})}\notag\\
%   &=\alpha(x^1_{t+1})\times\omega_t(\lambda^1_t,\sigma_t,z_{t+1},u_t)
%   \end{align}
\begin{align}
    &\frac{\sum_{x^2_{1:t}}\prob(x^1_{1:t+1},x^{2}_{1:t},u_{1:t},z_{1:t+1},\sigma_{1:t})}{\sum_{\Tilde{x}^1_{1:t+1}}\sum_{\Tilde{x}^{2}_{1:t}}\prob(\Tilde{x}^1_{1:t+1},\Tilde{x}^{2}_{1:t},u_{1:t},z_{1:t+1},\sigma_{1:t})}\notag\\
     &=\frac{\alpha(x^1_{t+1})\prob(z_{t+1}|z_t,u_t)\sigma_t(x^1_{1:t};u^1_t)\lambda^1_{t}(x^1_{1:t})}{\sum_{\Tilde{x}^1_{1:t+1}}\alpha(\Tilde{x}^1_{t+1})\prob(z_{t+1}|z_t,u_t)\sigma_t(\Tilde{x}^1_{1:t};u^1_t)\lambda^1_{t}(\Tilde{x}^1_{1:t})}\notag\\
    &\alpha(x^1_{t+1})\times\frac{\prob(z_{t+1}|z_t,u_t)\sigma_t(x^1_{1:t};u^1_t)\lambda^1_{t}(x^1_{1:t})}{\sum_{\Tilde{x}^1_{1:t+1}}\alpha(\Tilde{x}^1_{t+1})\prob(z_{t+1}|z_t,u_t)\sigma_t(\Tilde{x}^1_{1:t};u^1_t)\lambda^1_{t}(\Tilde{x}^1_{1:t})}\notag\\
    &=\alpha(x^1_{t+1})\times\frac{\prob(z_{t+1}|z_t,u_t)\sigma_t(x^1_{1:t};u^1_t)\lambda^1_{t}(x^1_{1:t})}{\sum_{\Tilde{x}^1_{1:t}}\prob(z_{t+1}|z_t,u_t)\sigma_t(\Tilde{x}^1_{1:t};u^1_t)\lambda^1_{t}(\Tilde{x}^1_{1:t})}\notag\\
    &=\alpha(x^1_{t+1})\times\frac{\sigma_t(x^1_{1:t};u^1_t)\lambda^1_{t}(x^1_{1:t})}{\sum_{\Tilde{x}^1_{1:t}}\sigma_t(\Tilde{x}^1_{1:t};u^1_t)\lambda^1_{t}(\Tilde{x}^1_{1:t})}
\end{align}
%   \begin{align}\label{eq:bayesupdate42}
%   \frac{\sum_{x^1_t}\prob(x^1_{t+1}|x^1_t,u_t)\gamma_t(x^1_t;u^1_t)\pi^1_{t}(x^1_t)}{\sum_{x^1_{t+1}}\sum_{x^1_t}\prob(x^1_{t+1}|x^1_t,u_t)\gamma_t(x^1_t;u^1_t)\pi^1_{t}(x^1_t)}
%   \end{align}
Therefore the belief update equation \eqref{eq:bayesupdat2} for $i=1,2$, can be written as
 \begin{align}
    %   \lambda^1_{t+1}(x^1_{1:t+1})=\alpha(x^1_{t+1})\times[\omega_t(\lambda^1_t,\sigma_t,u^1_t)](x^1_{1:t})
    \lambda^1_{t+1}(x^1_{1:t+1})=\alpha(x^1_{t+1})\times\tilde{\lambda}^1_t(x^1_{1:t}).
  \end{align}
  where $\tilde{\lambda}^1_t =\omega_t(\lambda^1_t,\sigma_t,u^1_t)$ is the belief on agent $1's$ state history until time $t$ after observing $u^1_t$ and $\omega$ is defined as follows:
  \begin{align}
      [\omega_t(\lambda^1_t,\sigma_t,u^1_t)](x^1_{1:t})=\frac{\sigma_t(x^1_{1:t};u^1_t)\lambda^1_{t}(x^1_{1:t})}{\sum_{\Tilde{x}^1_{1:t}}\sigma_t(\Tilde{x}^1_{1:t};u^1_t)\lambda^1_{t}(\Tilde{x}^1_{1:t})}
  \end{align}
  
%  Therefore the belief update equation \eqref{eq:bayesupdat2} for $i=1,2$, can be written as
%  \begin{align}
%       \lambda^1_{t+1}(x^1_{t+1})=\alpha(x^1_{t+1})\times\omega_t(\lambda^1_t,\sigma_t,z_{t+1},u_t)
%   \end{align}
% We denote the belief update equation using $\omega_t$.   
