# Supplementary material for: Optimal Symmetric Strategies in Multi-Agent Systems with Decentralized Information
Source: arXiv:2307.07150 source file (2023-07-14)
Supplement: Supplementary file 5 [file AppendixD.tex]

% \begin{proof}
\section{Proof of Lemma \ref{samestrategy}}\label{App:Lemma4}
% Let us consider the case where $\sum_{u'}\Phi_{t}^1(c_t; x,u')>0$ \red{Isn't the lemma only about the case where both phis sum up to be non-zero?}. 

Suppose that ${\sum_{u'^1}\Phi_{t}^1(c_t; x^1,u'^1)}> 0$ and ${\sum_{u'^2}\Phi_{t}^2(c_t; x^2,u'^2)}> 0$. Let $x^1 =x^2=x$ and $u^1=u^2=u$. Therefore by the definition of $\bar{g}^1$, we have
\begin{align}
&\bar{g}^1_{t}(x,c_t;u) := \frac{\Phi_{t}^1(c_t; x,u)}{\sum_{u'}\Phi_{t}^1(c_t; x,u')}\notag\\
%&=\prob(U^1_t=u \mid X^1_t=x, C_t=u_{1:t-1})\notag\\
    % &=\frac{\prob(U^1_t=u,X^1_t=x, C_t=u_{1:t-1})}{\sum_u\prob(U^1_t=u,X^1_t=x, C_t=u_{1:t-1})}\notag\\
%   &= \frac{\sum_{x^1_{1:t-1}}\Psi_{t}^1(c_t; x^1_{1:t-1}, x,u)}{\sum_{u'}\sum_{x'^1_{1:t-1}}\Psi_{t}^1(c_t; x'^1_{1:t-1}, x,u')}
&=\frac{\prob(U^1_t=u,X^1_t=x, C_t=u_{1:t-1})}{\sum_{u'}\prob(U^1_t=u',X^1_t=x, C_t=u_{1:t-1})}\notag\\
    &=\frac{\sum_{x_{1:t-1}}\prob(u,x,x_{1:t-1}, u_{1:t-1})}{\sum_{x'_{1:t-1}}\sum_{u'}\prob(u',x,x'_{1:t-1}, u_{1:t-1})}
   \label{eq:samestrategy1}
    \end{align}
    
    \red{I cannot follow the proof. Please rewrite clearly}
    For any realization $x,u,x_{1:t-1}$ and $u_{1:t-1}$ of $X^1_t,U^1_t,X_{1:t-1}$ and $C_t$ respectively. Considering the joint probability of random variables $U^1_t,X^1_t,X_{1:t-1}, C_t$ in \eqref{eq:samestrategy1},
    \begin{align}
    &\prob(U^1_t=u,X^1_t=x,X_{1:t-1}=x_{1:t-1}, C_t=u_{1:t-1})\notag\\
        &=\prob^g(u \mid x,x^1_{1:t-1},u_{1:t-1})\blue{\prob^f(x \mid x^1_{t-1}, u_{t-1})}\notag\\
    &\quad\times \prob^g(u^1_{t-1} \mid x^1_{1:t-1},c_{t-1})\prob^g(u^2_{t-1} \mid x^2_{1:t-1},c_{t-1})\notag\\
    &\quad\times\prob(x^1_{1:t-1}\mid c_{t-1})\prob(x^2_{1:t-1}\mid c_{t-1})\prob(c_{t-1})
    \end{align}
    
    % \red{the above equation is worng}
    % \begin{align}
    %     &=\sum_{x_{1:t-1}}\prob^g(U^1_t=u \mid X^1_{1:t},C_t)\prob^f(X^1_t=x \mid X^1_{t-1}, U_{t-1})\notag\\
    % &\quad\times \prob^g(U^1_{t-1} \mid X^1_{1:t-1},C_{t-1})\prob^g(U^2_{t-1} \mid X^2_{1:t-1},C_{t-1})\notag\\
    % &\quad\times\prob(X^1_{1:t-1}\mid C_{t-1})\prob(X^2_{1:t-1}\mid C_{t-1})
    % % &\frac{\times \prob^g(U^1_{t-1} \mid X^1_{1:t-1},C_{t-1})\prob^g(U^2_{t-1} \mid X^2_{1:t-1},C_{t-1})\prob(X^1_{1:t-1}\mid C_{t-1})\prob(X^2_{1:t-1}\mid C_{t-1})}{\sum_u\sum_{x_{1:t-1}}\prob^g(U^1_t=u \mid X^1_{1:t},C_t)\prob^f(X^1_t \mid X^1_{t-1}, U_{t-1})\prob^g(U^1_{t-1} \mid X^1_{1:t-1},C_{t-1})\times}\notag\\
    % % \times \prob^g(U^2_{t-1} \mid X^2_{1:t-1},C_{t-1})&\prob(X^1_{1:t-1}\mid C_{t-1})\prob(X^2_{1:t-1}\mid C_{t-1})
    % \end{align}
    % The denominator of \eqref{eq:samestrategy1} can be written as,
    % \begin{align}
    %     &\sum_u\sum_{x_{1:t-1}}\prob^g(U^1_t=u \mid X^1_{1:t},C_t)\prob^f(X^1_t \mid X^1_{t-1}, U_{t-1}) \notag\\
    % & \times \prob^g(U^1_{t-1} \mid X^1_{1:t-1},C_{t-1})\prob^g(U^2_{t-1} \mid X^2_{1:t-1},C_{t-1})\notag\\
    % & \times \prob(X^1_{1:t-1}\mid C_{t-1})\prob(X^2_{1:t-1}\mid C_{t-1})
    % \end{align}
Similarly for agent $2$ at time $t$, we consider the case where $\sum_{u'}\Phi_{t}^2(c_t; x,u')>0$. Therefore by the definition of $\bar{g}^2$, we have
\begin{align}
&\bar{g}^2_{t}(X_t^2=x,C_t=c_t;U_{t}^2=u) \doteq \frac{\Phi_{t}^2(c_t; x,u)}{\sum_{u'}\Phi_{t}^2(c_t; x,u')}\notag\\
    &=\frac{\prob(U^2_t=u,X^2_t=x, C_t=u_{1:t-1})}{\sum_u\prob(U^2_t=u,X^2_t=x, C_t=u_{1:t-1})}\notag\\
    &=\frac{\sum_{x_{1:t-1}}\prob(u,x,x_{1:t-1}, u_{1:t-1})}{\sum_{x_{1:t-1}}\sum_{u'}\prob(u',x,x_{1:t-1}, u_{1:t-1})}\label{samestrategy1}
    \end{align}
    For any realization $x,u,x_{1:t-1},u_{1:t-1}$ of $X^2_t,U^2_t,X_{1:t-1}$ and $C_t$ respectively. The joint probability of random variables $U^2_t,X^2_t,X_{1:t-1}, C_t$ in \eqref{samestrategy1} can be written as,
    \begin{align}
        &=\prob^g(u \mid x,x^2_{1:t-1},u_{1:t-1})\prob^f(x \mid x^2_{t-1}, u_{t-1})\notag\\
    &\times \prob^g(u^2_{t-1} \mid x^2_{1:t-1},c_{t-1})\prob^g(u^1_{t-1} \mid x^1_{1:t-1},c_{t-1})\notag\\
    &\times\prob(x^2_{1:t-1}\mid c_{t-1})\prob(x^1_{1:t-1}\mid c_{t-1})\prob(c_{t-1})
    \end{align}
    % The denominator of \eqref{samestrategy1} can be written as,
    % \begin{align}
    %     &\sum_u\sum_{x_{1:t-1}}\prob^g(U^2_t=u \mid X^2_{1:t},C_t)\prob^f(X^2_t \mid X^2_{t-1}, U_{t-1}) \notag\\
    % & \times \prob^g(U^2_{t-1} \mid X^2_{1:t-1},C_{t-1})\prob^g(U^1_{t-1} \mid X^1_{1:t-1},C_{t-1})\notag\\
    % & \times \prob(X^2_{1:t-1}\mid C_{t-1})\prob(X^1_{1:t-1}\mid C_{t-1})
    % \end{align}
% \end{proof}
Using symmetric system dynamics and strategies for both the agents, the ratio %of $\phi(.)$
is same for both the agents. \red{Not at all clear why this statement is true}

For the cases where one of the distribution ${\sum_{u'}\Phi_{t}^1(c_t; x,u')}=0$ or ${\sum_{u'}\Phi_{t}^2(c_t; x,u')}=0$, at time $t$. It is straight forward to see from the definitions of $\bar{g}^1_{t}$ and $\bar{g}^2_{t}$ that the ratio is same for both the agents. Therefore  control strategy $\bar{g}^1=\bar{g}^2=:\bar{g}$ at all time $t$.

% \begin{align*}
%     &\pi_{t+1}(x_{t+1})=\prob(X_{t+1}=x_{t+1}|u_{1:t},\gamma_{1:t})\notag\\
%     &=\frac{\prob(X_{t+1}=x_{t+1},U_t=u_t|u_{1:t-1},\gamma_{1:t})}{\prob(U_t=u_t|u_{1:t-1},\gamma_{1:t})}\notag\\
%     &=\frac{\sum_{x_t}\prob(x_{t+1},x_t,u_t|u_{1:t-1},\gamma_{1:t})}{\sum_{x_{t+1}}\sum_{x_t}\prob(x_{t+1},x_t,u_t|u_{1:t-1},\gamma_{1:t})}\notag\\
%     &=\frac{\sum_{x_t}\prob(x^1_{t+1}|x^1_t,u_t)\prob(x^2_{t+1}|x^2_t,u_t)\gamma_t(x^1_t;u^1_t)\gamma_t(x^2_t;u^2_t)\prob(x_t|u_{1:t-1},\gamma_{1:t})}{\sum_{x_{t+1}}\sum_{x_t}\prob(x^1_{t+1}|x^1_t,u_t)\prob(x^2_{t+1}|x^2_t,u_t)\gamma^1_t(x^1_t;u^1_t)\gamma^2_t(x^2_t;u^2_t)\prob(x_t|u_{1:t-1},\gamma_{1:t})}\notag\\
%     &\stackrel{(a)}{=}\frac{\sum_{x_t}\prob(x^1_{t+1}|x^1_t,u_t)\prob(x^2_{t+1}|x^2_t,u_t)\gamma_t(x^1_t;u^1_t)\gamma_t(x^2_t;u^2_t)\prob(x_t|u_{1:t-1},\gamma_{1:t-1})}{\sum_{x_{t+1}}\sum_{x_t}\prob(x^1_{t+1}|x^1_t,u_t)\prob(x^2_{t+1}|x^2_t,u_t)\gamma_t(x^1_t;u^1_t)\gamma_t(x^2_t;u^2_t)\prob(x_t|u_{1:t-1},\gamma_{1:t-1})}\notag\\
%     &\stackrel{(b)}{=}\frac{\sum_{x_t}\prob(x^1_{t+1}|x^1_t,u_t)\prob(x^2_{t+1}|x^2_t,u_t)\gamma_t(x^1_t;u^1_t)\gamma_t(x^2_t;u^2_t)\pi_{t}(x_t)}{\sum_{x_{t+1}}\sum_{x_t}\prob(x^1_{t+1}|x^1_t,u_t)\prob(x^2_{t+1}|x^2_t,u_t)\gamma_t(x^1_t;u^1_t)\gamma_t(x^2_t;u^2_t)\pi_{t}(x_t)}\notag\\
%     &=\eta_t( \Pi_{t},\Gamma_t,U_t)
% \end{align*}
